# Supplementary material for: Observation of Subnatural-Linewidth Biphotons In a Two-Level Atomic Ensemble
Source: arXiv:2501.11908 source file (2025-01-21)
Supplement: Supplementary file 1 [file appendix.tex]

\appendix

\section{Biphoton Wave Packet and the Glauber Correlation Function}

In the perturbation theory, the biphoton state is given by

\begin{equation}
\left|\Psi\right\rangle =-\frac{i}{\hbar}\sideset{}{_{-\infty}^{+\infty}}\int dt\hat{H}_{I}(t)\left|0\right\rangle ,\label{eq:A1}
\end{equation}
where the interaction Hamiltonian is

\begin{equation}
H_{I}=\frac{\varepsilon_{0}A}{2}\sideset{}{_{-L/2}^{+L/2}}\int dz\chi^{(3)}E_{p}^{(+)}E_{p}^{(+)}\hat{E}_{s}^{(-)}\hat{E}_{as}^{(-)}+H.c.,\label{eq:A2}
\end{equation}
with $A$ being the single-mode cross-section area, in which the generated fields are collected for the correlation measurement, and $L$ the length of the atomic ensemble. The positive-frequency part of the pump field is described by

\begin{equation}
E_{p}^{(+)}(z,t)=E_{p}e^{i(k_{p}z-\omega_{p}t)},\label{eq:A3}
\end{equation}
where $E_{p}$ is the corresponding electric field's amplitude. $\hat{E}_{s}^{(-)}$ and $\hat{E}_{as}^{(-)}$ are the single-transverse-mode operators of the Stokes and anti-Stokes fields,

\begin{equation}
\begin{array}{c}
\hat{E}_{s}^{(-)}(z,t)=\sqrt{\frac{\hbar\varpi_{s}}{c\varepsilon_{0}A\pi}}\int d\omega\hat{a}_{s}^{\dagger}(\omega)e^{i(k_{s}(\omega)z-\omega t)}\\
\\
\hat{E}_{as}^{(-)}(z,t)=\sqrt{\frac{\hbar\varpi_{as}}{c\varepsilon_{0}A\pi}}\int d\omega\hat{a}_{as}^{\dagger}(\omega)e^{i(k_{as}(\omega)z-\omega t)}
\end{array},
\label{eq:A4}
\end{equation}
Here, $\hat{a}_{s}^{\dagger}(\omega)$ and $\hat{a}_{as}^{\dagger}(\omega)$ are the creation operators of the Stokes and anti-Stokes fields, respectively, which obey the commutation relations $\left[\hat{a}_{s}(\omega), \hat{a}_{s}^{\dagger}(\omega^{'})\right]=\left[\hat{a}_{as}(\omega), \hat{a}_{as}^{\dagger}(\omega^{'})\right]=\delta(\omega-\omega^{'})$, and $\varpi_{s}(\varpi_{as})$ is the center frequency of the Stokes (anti-Stokes) field.

By using Eq.\ref{eq:A3} and Eq.\ref{eq:A4}, the interaction Hamiltonian and biphoton wave function can be obtained as follows.

\begin{equation}
\begin{array}{ccc}
H_{I} & = & \frac{i\hbar L}{2\pi}\int d\omega_{s}d\omega_{as}\kappa(\omega_{as},\omega_{s}){\rm sinc}(\frac{\Delta kL}{2})\\
\\
 &  & \times\hat{a}_{as}^{\dagger}(\omega_{as})\hat{a}_{s}^{\dagger}(\omega_{s})e^{-i(\omega_{p}+\omega_{p}-\omega_{as}-\omega_{s})t}+H.c.,
\end{array}\label{eq:A5}
\end{equation}

\begin{equation}
\begin{array}{ccc}
\left|\Psi\right\rangle  & = & L\int d\omega_{as}\kappa(\omega_{as},\omega_{p}+\omega_{p}-\omega_{as}){\rm sinc}(\frac{\Delta kL}{2})\\
\\
 &  & \times\hat{a}_{as}^{\dagger}(\omega_{as})\hat{a}_{s}^{\dagger}(\omega_{p}+\omega_{p}-\omega_{as})\left|0\right\rangle 
\end{array}\label{eq:A6}
\end{equation}

where $\Delta k=k_{as}-k_{s}-(k_{p}+k_{p})$ is the phase mismatch, $\kappa(\omega_{as})=\chi_{as}^{(3)}E_{p0}E_{p0}\sqrt{\varpi_{as}\varpi_{s}}/(2ic)$ is the nonlinear parametric coupling coefficient, and

\begin{equation}
\begin{array}{cc}
\chi_{as}^{(3)}=\frac{N\left|\mu_{eg}\right|^{4}}{4\hbar^{3}\varepsilon_{0}(\Delta-i\gamma_{e})} & [\frac{1}{(\Delta-\delta+i\gamma_{e})(-\delta+i\gamma_{g})}\\
\\
 & +\frac{1}{(\Delta-\delta-i\gamma_{e})(\delta+i\gamma_{g})}]
\end{array}\label{eq:A7}
\end{equation}
is the third-order nonlinear susceptibility. Here, $N$ is the atomic
density, $\gamma_{e}$ is the population relaxation rate of the excited
state $\left|e\right\rangle $, $\gamma_{g}$ is the dephasing rate
of the inhomogeneously broadened ground state, and $\mu_{eg}$ is the
atomic dipole moment associated with the transition $\left|e\right\rangle \longleftrightarrow\left|g\right\rangle $.

The Glauber correlation function is defined by

\begin{equation}
\begin{array}{c}
G^{(2)}(\tau)\\
\\
\\
\end{array}\begin{array}{c}
=\\
\\
=
\end{array}\begin{array}{l}
\left\langle \Psi\right|\hat{a}_{s}^{\dagger}(t_{s})\hat{a}_{as}^{\dagger}(t_{as})\hat{a}_{as}(t_{as})\hat{a}_{s}(t_{s})\left|\Psi\right\rangle \\
\\
\left|\Psi(t_{as},t_{s})\right|^{2}
\end{array}\label{eq:A8}
\end{equation}
Here, $\hat{a}_{s}(\omega)$ and $\hat{a}_{as}(\omega)$ are the annihilation operators of the Stokes and anti-Stokes fields, respectively. $\Psi(t_{as},t_{s})$ is the biphoton wave function in the time domain,
\[
\Psi(t_{as},t_{s})=\psi(\tau)e^{-i(\omega_{p}+\omega_{p})t_{s}},
\]
where 

\begin{equation}
\psi(\tau)=\frac{L}{2\pi}\int d\omega_{as}\Phi(\omega_{as})\kappa(\omega_{as})e^{(-i\omega_{as}\tau)},\label{eq:A9}
\end{equation}

with $\tau=t_{as}-t_{s}$ being the time delay between the detection of the anti-Stokes and Stokes photons, and $\Phi(\omega_{as})$ the longitudinal detuning function,

\begin{equation}
\Phi(\omega_{as})={\rm sinc}(\frac{L}{2}\Delta k)e^{i(k_{as}+k_{s})\frac{L}{2}}.\label{eq:A10}
\end{equation}

In this work, the biphoton wave function is dominated by $\kappa(\omega_{as})$, which is associated with the third-order nonlinear susceptibility $\chi_{as}^{(3)}$, so that

\begin{equation}
\Psi(\tau)\simeq-\frac{i\sqrt{\varpi_{as}\varpi_{s}}E_{p0}E_{p0}L}{\sqrt{8\pi}c}\int d\omega_{as}\chi_{as}^{(3)}e^{(-i\omega_{as}\tau)}.\label{eq:A11}
\end{equation}

The Glauber correlation function can then be evaluated to be

\begin{equation}
G^{(2)}(\tau)\propto[e^{-2\gamma_{e}\tau}+e^{-2\gamma_{g}\tau}-2{\rm cos}(\varOmega_{e}\tau)e^{-(\gamma_{e}+\gamma_{g})\tau}]\Theta(\tau),\label{eq:A12}
\end{equation}

where $\Theta(\tau)$ is the Heaviside step function and $\varOmega_{e}$ is the effective Rabi frequency $\varOmega_{e}=\sqrt{\Delta^{2}+\left|\varOmega_{p}\right|^{2}}$.

\begin{figure}
\includegraphics[width=8cm,height=5cm]{magnetic.eps}
\caption{\label{fig:9}The ground-state decoherence rate versus the magnetic field of the magneto-optical trap.}
\end{figure}

\section{Dependence of the Biphoton linewidth on dephasing rate}
As mentioned above, the biphoton bandwidth is only limited by the ground-state decoherence in the presence of the inhomogeneous magnetic field resulting from the magneto-optical trap. It is thus possible to generate narrower biphoton bandwidth by switching off the magnetic field during the biphoton generation. Instead of completely switching off the magnetic field from the trapping coils, we demonstrate that the bandwidth of the biphotons can gradually be reduced by decreasing the inhomogeneous magnetic field of the magneto-optical trap. Since the moderate OD is required to generate the sub-natural linewidth biphotons in a two-level atomic ensemble, the system can be kept in the same OD even though the magnetic field for trapping is smaller. As shown in Fig.\ref{fig:7}, the ground-state decoherence rate can be gradually reduced by decreasing the inhomogeneous magnetic field of the magneto-optical trap at the same OD. A direct or complete switch-off of our magnetic field will require additional electronic device because in this switching-like method we have to increase the timing sequence for each measurement in order to protect the power supply from being damaged.
